# Supplementary material for: Mining the Minoria: Unknown, Under-represented, and Under-performing Minority Groups
Source: arXiv:2411.04761 source file (2025-04-21)
Supplement: Supplementary file 1 [file appendix.tex]

\section{\yoom Mining in Higher Dimensions -- Extended Results}
